# Supplementary material for: Petrov-Galerkin Dynamical Low Rank Approximation:SUPG stabilisation of advection-dominated problems
Source: arXiv:2407.01404 source file (2024-07-01)
Supplement: Supplementary file 1 [file si-norm-stab-old.tex]

As the implicit Euler is an impractical algorithm for DLR schemes due to its very coupled nature, we are interested in using other time-integration schemes that to reach a balance between computability and desirable stability properties. One such choice is given by the semi-implicit time-stepping scheme. The desirable properties of this scheme become apparent under moderate stochasticity; we make the following assumtions: 
\begin{gather}
	\varepsilon^{\star}(\omega) \leq C_1 \varepsilon(\omega) \label{eqn:varepscond} \\
	|c^{\star}(x, \omega)| \leq \sqrt{1 - \delta} |c(x, \omega)| \label{eqn:cstarcond},
\end{gather}
and we furthermore assume that $\bu$ is divergence-free, i.e., $\nabla \cdot \bu = 0$. 

In what follows, we establish norm-stability bounds for the numerical solution under a hyperbolic CFL condition as well as a condition on $\delta_K$.

%TODO: likely something wrong with the max-mins
%TODO: is the Volker bound the same idea, but a slightly sharper bound of Gronwall type?
%TODO: remarks about the special case when div(b) = 0. 

\begin{theorem}
	For a general advection-diffusion-reaction operator such that TODO, TODO and TODO hold; then, for
	\begin{equation} \label{eqn:deltaK-si-cond}
		\delta_K \leq \cdots
	\end{equation}
	the iterates $\{\uhr[k]\}_{k=0}^N$ satisfy
	\begin{equation} \label{eqn:si-bound}
		a \leq b
	\end{equation}
\end{theorem}
\begin{proof}
	We test~\eqref{eqn:varf-adr-disc-si} against $\uhr[n+1]$. 
	The first term is developped as usual, 
	\[
		\frac{1}{2\dt}(\|\uhr[n+1] \|_{X,\Lthm}^2 -  \| \uhr[n] \|_{X,\Lthm}^2 +  \| \uhr[n+1]- \uhr[n] \|_{X,\Lthm}^2). 
	\]
	We then add and subtract the quantity
	\begin{equation}
		(\varepsilon^{\star} \nabla \uhr[n+1], \nabla v_{\hhmu}) + (c^{\star} \uhr[n+1], v_{\hhmu}) + \sum_{K \in \Th} (- \varepsilon^{\star} \Delta \uhr[n+1] + c^{\star} \uhr[n+1], \bu \cdot \nabla v_{\hhmu})_K, 
	\end{equation}
	allowing us to recover the variational formulation of the implicit Euler with some extra terms: 
	\begin{multline*}
		\frac{1}{2\dt}(\|\uhr[n+1] \|_{X,\Lthm}^2 -  \| \uhr[n] \|_{X,\Lthm}^2 +  \| \uhr[n+1]- \uhr[n] \|_{X,\Lthm}^2) + \aSUPG(\uhr[n+1], \uhr[n+1])
		\\ 
		+ \sum_{K \in \Th} \frac{\delta_K}{\dt} (\uhr[n+1] - \uhr[n], \bu \cdot \nabla \uhr[n+1]) = (f, \uhr[n+1]) + \sum_{K \in \Th} \delta_K (f, \bu \cdot \nabla \uhr[n+1]) 
		\\ + (\varepsilon^{\star} \nabla (\uhr[n+1] - \uhr[n]), \nabla \uhr[n+1]) + (c^{\star} (\uhr[n+1] - \uhr[n]), \uhr[n+1]) 
		\\ 
		+ \sum_{K \in \Th} \delta_K (- \varepsilon^{\star} \Delta(\uhr[n+1] - \uhr[n]) + c^{\star} (\uhr[n+1] - \uhr[n]), \bu \cdot \nabla \uhr[n+1])_K
	\end{multline*}
	We then bound the following terms: 
	\begin{align}
		|(\varepsilon^{\star} \nabla (\uhr[n+1] - \uhr[n]), \nabla \uhr[n+1])| &\leq \frac{C_I^2}{2 h^2} \|\uhr[n+1] - \uhr[n]\|_{X,\Lthm}^2 + \frac{C_1 }{2} \| \varepsilon\nabla \uhr[n+1]\|^2_{X, \Lthm}
		\\
		|(c^{\star} (\uhr[n+1] - \uhr[n]), \uhr[n+1])| &\leq \frac{1}{2}\|\uhr[n+1] - \uhr[n]\|_{X,\Lthm}^2 +\frac{1}{2}\|c^{\star} \uhr[n+1] \|^2_{X, \Lthm}  \\
		|(- \varepsilon^{\star} \Delta (\uhr[n+1]- \uhr[n]), \bu \cdot \nabla \uhr[n+1])_K| &\leq \trnorm{\varepsilon^{\star}}_K \frac{C_I^4}{h^4} \|\uhr[n+1] - \uhr[n]\|^2_{K,\Lthm} + \|\bu \cdot \nabla \uhr[n+1]\|^2_{K,\Lthm}
		\\
		|(c^{\star} (\uhr[n+1] - \uhr[n]), \bu \cdot \nabla \uhr[n+1])_K| &\leq \frac{1}{2} \trnorm{c^{\star}}_K \|\uhr[n+1] - \uhr[n]\|_{K,\Lthm}^2 +\frac{1}{2}\|\bu \cdot \nabla  \uhr[n+1] \|^2_{K, \Lthm} 
	\end{align}
	Furthermore, we have that
	\begin{gather}
		|(f, \uhr[n+1])| \leq \| \mu^{-1/2} f\|_{X,\Lthm} \|\mu^{1/2}\uhr[n+1] \|_{X,\Lthm} \leq \frac{1}{2\mu_0} \|f\|^2_{X, \Lthm} + \frac{1}{2}\| \mu^{1/2} \uhr[n+1] \|^2_{X, \Lthm} 
		\\
		\delta_K |(f, \bu \cdot \nabla \uhr[n+1])_K| \leq \frac{\delta_K}{2} \|f\|^2_{K,\Lthm} + \frac{\delta_K}{2} \| \bu \cdot \nabla \uhr[n+1] \|^2_{K,\Lthm}
	\end{gather}

\end{proof}
%TODO: the first line, something fishy...
%TODO: need to change the trnorm notation
%TODO: also the _K notation. 
